# Supplementary material for: Catch Missing Details: Image Reconstruction with Frequency Augmented Variational Autoencoder
Source: arXiv:2305.02541 source file (2023-11-03)
Supplement: Supplementary file 2 [file imagenet_recon_supp.tex]

\begin{figure*}[t!]
    % \centerline{
    \subfloat{\includegraphics[width=1.0\textwidth]{cvpr2023/latex/figures/supplement/supp-imagenet-recon-1.pdf}}\\
    \subfloat{\includegraphics[width=1.0\textwidth]{cvpr2023/latex/figures/supplement/supp-imagenet-recon-2.pdf}}\\
    % \captionsetup{aboveskip=3pt}
    \caption{\small ImageNet reconstruction. VQ-GAN with downsampling factor $f=4$ is from \cite{taming}, VQ-GAN with $f=16$ is from \cite{latent-diffusion}. DALL-E is from \cite{dalle}. The labels for each row of images are: goldfish, tiger, gray whale, Egyptian cat, African elephant, papillon.
    }
    \label{fig:supp-imagenet-recon}
    \vspace{-0.5cm}
\end{figure*}

% Visualization on CelebA-HQ dataset for the ablation studies in Table 2 of the paper. $\text{Ours}^{*}$ is FA-VAE model with FCM and FFL, no DSL. $\text{Ours}^{**}$ is FA-VAE model with FCM with SL without gaussian filters. $\text{DSL}^{*}$ is DSL with non pair-wise sigmas. VQ-GAN is from \cite{taming}
