# Supplementary material for: Catch Missing Details: Image Reconstruction with Frequency Augmented Variational Autoencoder
Source: arXiv:2305.02541 source file (2023-11-03)
Supplement: Supplementary file 3 [file supp_favae_settings.tex]

\begin{table*}\centering
\footnotesize
\setlength{\tabcolsep}{2.2mm}
\begin{tabular}{l | c c c c c c c c c}
\toprule
Dataset & $f$ & Channel Multiplier & dropout & attn resolution & FFL weight $\alpha$ & DSL Weight $\beta$ & Disc weight & $|\mathfrak{C}|$ & $n_z$  \\
\midrule
CelebA-HQ \cite{celeba-hq}    & 16    & [1,1,2,2,4] & 0.0 & [16] & 1.0 & 0.01 & 0.75 & 1024 & 256\\
ImageNet \cite{imagenet}   & 4     & [1,2,4] & 0.0 & [] & 1.0 & 0.01 & 0.75  & 8192 & 3\\
ImageNet \cite{imagenet}    & 16    & [1,1,2,2,4] & 0.0 & [16] & 1.0 & 0.01 & 0.75 & 16384 & 256 \\
FFHQ \cite{ffhq}    & 16    & [1,1,2,2,4] & 0.0 & [16] & 1.0 & 0.01 & 0.75 & 2048 & 256 \\

\bottomrule
\end{tabular}
\caption{Hyperparameters and FA-VAE'settings for codebook training.}
\vspace{-0.5cm}
\label{tab:supp_favae}
\end{table*}
